# Supplementary material for: Flatness-Aware Minimization for Domain Generalization
Source: arXiv:2307.11108 source file (2023-07-20)
Supplement: Supplementary file 1 [file appendix_vis.tex]

\section{Visulization}
